# Supplementary material for: Effective Learning of Probabilistic Models for Clinical Predictions from Longitudinal Data
Source: arXiv:1811.00749 source file (2018-11-02)
Supplement: Supplementary file 1 [file appendix2.tex]

\chapter{Appendix B}
\label{appendix:b}
\begin{mydef}~\ref{amalg_noisyor}
	Given a set of CIMs associated with multiple RCTBN clauses, the amalgamation operation (addition) on the CIMs will result in a consistent homogeneous Markov process. The amalgamation operation is equivalent to applying the Noisy-Or combining rule to these RCTBN clauses.   
\end{mydef}
\begin{proof}
In order to prove this theory, take the medical diagnosis as an example, define the predicates and Bayesian logic clauses as:
\begin{align*}
& domain (CVD/1, discrete, [true, false])\\ \nonumber
& domain (Ascendant/2, discrete, [true, false])\\ \nonumber
& domain (Hypertension/1, discrete, [true, false])\\ \nonumber
& domain (BMI/1, discrete, [healthy, unhealthy])
\end{align*}
%Assume there are two Bayesian logic clauses:
\begin{equation*}
\textit{CVD}(X) | \textit{Ascendant} (Y,X), \textit{Hypertension}(Y) \\ \nonumber
\end{equation*}
\begin{equation*}
\textit{CVD}(X) | \textit{BMI} (X)
\end{equation*}
%\begin{align*}
%& \textit{CVD}(X) | \textit{Ascendant} (Y,X), \textit{Hypertension}(Y) \\ \nonumber
%& \textit{CVD}(X) | \textit{BMI} (X)
%\end{align*}
The first logic rule means if a person ($X$) has an ascendant ($Y$) who has high blood pressure, then there is a conditional intensity matrix describing the probability distributions of $X$ having cardiovascular disease(CVD) over its trajectory. The second logic rule means the trajectory of a person having CVD stochastically depends on the trajectory of his body mass index(BMI). 
%The CIM of each clause can be specified by domain knowledge or learned from the data set through the process similar as the propositional CTBN introduced in \textbf{Chapter}~\ref{chap1}.
Since $\textit{Ascendant} (Y,X)$ is an existential predicate, we can omit it when specify the CIMs. For simplification, denote MICs $Q_{CVD_x|Hyp_y^i}$ and $Q_{CVD_x|BMI_x^i}$ as: 

%So, the CIMs can be denoted as:\\
%$Q_{Dia_x|Dia_y^i} (i=0,1,2)=
%\begin{bmatrix}
%  -q_{Dia_x^0|Dia_y^i} & q_{Dia_x^0Dia_x^1|Dia_y^i} & q_{Dia_x^0Dia_x^2|Dia_y^i} \\
%  q_{Dia_x^1Dia_x^0|Dia_y^i} & -q_{Dia_x^1|Dia_y^i}  & q_{Dia_x^1Dia_x^2|Dia_y^i} \\
%  q_{Dia_x^2Dia_x^0|Dia_y^i}& q_{Dia_x^2Dia_x^1|Dia_y^i} & -q_{Dia_x^2|Dia_y^i} 
%\end{bmatrix}$\\

%$Q_{CVD_x|Hyp_y^i} =
%\begin{bmatrix}
%  -q_{CVD_x^0|Hyp_y^i} & q_{CVD_x^0CVD_x^1|Hyp_y^i} \\
%  q_{CVD_x^1CVD_x^0|Hyp_y^i} & -q_{CVD_x^1|Hyp_y^i}  
%\end{bmatrix}$\
%Where $i=0, 1$. Similarly, the MICs for the second clause is\\
%$Q_{CVD_x|BMI_x^i} =
%\begin{bmatrix}
%  -q_{CVD_x^0|BMI_x^i} & q_{CVD_x^0CVD_x^1|BMI_x^i} \\
%  q_{CVD_x^1CVD_x^0|BMI_x^i} & -q_{CVD_x^1|BMI_x^i}
%\end{bmatrix}$\

$\begin{bmatrix}
-q_{a^i}^{11} & q_{a^i}^{12} \\
q_{a^i}^{21} & -q_{a^i}^{22} 
\end{bmatrix}$\ 
and 
$\begin{bmatrix}
-q_{b^i}^{11} & q_{b^i}^{12} \\
q_{b^i}^{21} & -q_{b^i}^{22} 
\end{bmatrix}$\ respectively.\\

Consider the variable ordering
$[CVD_x,Hyp_y,BMI_x]$, the $Q_{CVD_x|Hyp_y^i}$ can be expanded over the variable set $\{CVD_x,Hyp_y,BMI_x\}$ based on the definition of  amalgamation~\cite{Nodelmanthesis} as:

$\begin{bmatrix}
-q_{a^0}^{11} & q_{a^0}^{12} & 0 & 0 & 0 & 0 & 0 & 0\\
q_{a^0}^{21} & -q_{a^0}^{22} & 0 & 0 & 0 & 0 & 0 & 0\\
0 & 0 & -q_{a^1}^{11} & q_{a^1}^{12}&  0 & 0 & 0 & 0\\
0 & 0 & q_{a^1}^{21} & -q_{a^1}^{22}& 0 & 0 & 0 & 0 \\
0 & 0 & 0 & 0 & -q_{a^0}^{11} & q_{a^0}^{12} & 0 & 0\\
0 & 0 & 0 & 0 & q_{a^0}^{21} & -q_{a^0}^{22} & 0 & 0\\
0 & 0 & 0 & 0 & 0 & 0 & -q_{a^1}^{11} & q_{a^1}^{12}  \\
0 & 0 & 0 & 0 & 0 & 0 & q_{a^1}^{21} & -q_{a^1}^{22} \\  
\end{bmatrix}$\\

Similarly, the $Q_{CVD_x|BMI_x^i}$ can be expanded as:\\
$\begin{bmatrix}
-q_{b^0}^{11} & q_{b^0}^{12} & 0 & 0 & 0 & 0 & 0 & 0\\
q_{b^0}^{21} & -q_{b^0}^{22} & 0 & 0 & 0 & 0 & 0 & 0\\
0 & 0 & -q_{b^0}^{11} & q_{b^0}^{12}&  0 & 0 & 0 & 0\\
0 & 0 & q_{b^0}^{21} & -q_{b^0}^{22}& 0 & 0 & 0 & 0 \\
0 & 0 & 0 & 0 & -q_{b^1}^{11} & q_{b^1}^{12} & 0 & 0\\
0 & 0 & 0 & 0 & q_{b^1}^{21} & -q_{b^1}^{22} & 0 & 0\\
0 & 0 & 0 & 0 & 0 & 0 & -q_{b^1}^{11} & q_{b^1}^{12}  \\
0 & 0 & 0 & 0 & 0 & 0 & q_{b^1}^{21} & -q_{b^1}^{22} \\  
\end{bmatrix}$\\

Denote $Q_{Hyp_y}$ and $Q_{BMI_x}$ as\\
$\begin{bmatrix}
-q^{a^0} & q^{a^0a^1} \\
q^{a^1a^0} & -q^{a^1} 
\end{bmatrix}$\, 
$\begin{bmatrix}
-q^{b^0} & q^{b^0b^1} \\
q^{b^1b^0} & -q^{b^1} 
\end{bmatrix}$\\

These two CIMs can be expanded as:\\
$\begin{bmatrix}
\fontsize{4.5pt}{-1em}
-q^{a^0} & 0 & q^{a^0a^1} & 0 & 0 & 0 & 0 & 0\\
0 & -q^{a^0} & 0 & q^{a^0a^1} & 0 & 0 & 0 & 0\\
q^{a^1a^0} & 0 & -q^{a^1} & 0 & 0 & 0 & 0 & 0\\
0 & q^{a^1a^0} & 0 & -q^{a^1} & 0 & 0 & 0 & 0 \\
0 & 0 & 0 & 0 & -q^{a^0} & 0 & q^{a^0a^1} & 0\\
0 & 0 & 0 & 0 & 0 & -q^{a^0} & 0 & q^{a^0a^1}\\
0 & 0 & 0 & 0 & q^{a^1a^0} & 0 & -q^{a^1} & 0\\
0 & 0 & 0 & 0 & 0 & q^{a^1a^0} & 0 & -q^{a^1}\\
\end{bmatrix}$\\
$\begin{bmatrix}
-q^{b^0} & 0 & 0 & 0 &q^{b^0b^1} & 0 & 0 & 0\\
0 & -q^{b^0} & 0 & 0 & 0 &q^{b^0b^1} & 0 & 0\\
0 & 0 & -q^{b^0} & 0 & 0 & 0 &q^{b^0b^1} & 0\\
0 & 0 & 0 & -q^{b^0} & 0 & 0 & 0 &q^{b^0b^1}\\
q^{b^1b^0} & 0 & 0 & 0 & -q^{b^1} & 0 & 0 & 0\\
0 & q^{b^1b^0} & 0 & 0 & 0 & -q^{b^1} & 0 & 0\\
0 & 0 & q^{b^1b^0} & 0 & 0 & 0 & -q^{b^1} & 0\\
0 & 0 & 0 & q^{b^1b^0} & 0 & 0 & 0 & -q^{b^1}\\
\end{bmatrix}$\ \\

According to the amalgamation operation~\cite{Nodelmanthesis}, the intensity matrix of the corresponding homogeneous Markov process would be the matrix shown in \textbf{Fig.}~\ref{amalg2}. As it shows, the corresponding homogeneous Markov process is consistent with the CTBN constraint because any entry in the matrix corresponding to multiple transitions is zero. The diagonal elements are the sum of the diagonal entries of the same row from each expanded CIM over all variables. It can be interpreted as that each CIM specified a trajectory of the corresponding variable which is competing with other variables' transitions, the transition happening first would dominate the joint trajectory. According to the properties of exponential distribution \textit{``if $T_1$ and $T_2$ are distributed exponentially with parameters $q_1$ and $q_2$, define $T_c = min\{T_1, T_2\}$, then $T_c$ is distributed exponentially with parameter $q_c = q_1 + q_2$''}. The joint trajectory is still exponential distribution with the sum over all competing transition intensities as the parameters on the diagonal of the matrix after amalgamation. Here, the two Bayesian clauses are assumed to be two competing transitions of the same variable but under two different casual influences. So the resulting transition time of such variable is the shorter time between these two transition distributions. However, the Markov process over this joint transition matrix no long has the unique minimal S-map CTBN like the traditional amalgamation~\cite{Nodelmanthesis}, since it involves the summations of off-diagonal intensities when amalgamation over the expanded CIMs for the same variable but different parents (i.e. multiple Bayesian clauses with the same head). 
\begin{sidewaysfigure}
%\begin{figure*}[htbp]
	\advance\leftskip-2.5cm
	%\begin{widetext}
	%\begin{minipage}[H]{2\textwidth}
	%\begin{multicols}{1}
	%\tiny
	\fontsize{4pt}{-1em}
	%\begin{sideways} 
	$\begin{bmatrix}
	\fontsize{4.5pt}{-1em} 
	-q_{a^0}^{11}-q_{b^0}^{11}-q^{a^0}-q^{b^0}&q_{a^0}^{12}+q_{b^0}^{12}&q^{a^0a^1}&0&q^{b^0b^1}&0&0&0\\
	q_{a^0}^{21}+ q_{b^0}^{21}&-q_{a^0}^{22}-q_{b^0}^{22}-q^{a^0}-q^{b^0}&0 & q^{a^0a^1} & 0 & q^{b^0b^1} & 0 & 0\\
	q^{a^1a^0}& 0 & -q_{a^1}^{11}-q_{b^0}^{11}-q^{a^1}-q^{b^0}& q_{a^1}^{12}+q_{b^0}^{12}&  0 & 0 & q^{b^0b^1} & 0\\
	0& q^{a^1a^0} & q_{a^1}^{21}+q_{b^0}^{21} & -q_{a^1}^{22}-q_{b^0}^{22}-q^{a^1}-q^{b^0}& 0 & 0 & 0 & q^{b^0b^1} \\
	q^{b^1b^0}& 0 & 0 & 0 & -q_{a^0}^{11}-q_{b^1}^{11}-q^{a^0}-q^{b^1}  & q_{a^0}^{12}+q_{b^1}^{12} & q^{a^0a^1} & 0\\
	0& q^{b^1b^0} & 0 & 0 & q_{a^0}^{21}+q_{b^1}^{21} & -q_{a^0}^{22}-q_{b^1}^{22}-q^{a^0}-q^{b^1} & 0 & q^{a^0a^1}\\
	0& 0 & q^{b^1b^0} & 0 & q^{a^1a^0} & 0 & -q_{a^1}^{11}-q_{b^1}^{11}-q^{a^1}-q^{b^1} & q_{a^1}^{12}+q_{b^1}^{12} \\
	0& 0 & 0 & q^{b^1b^0} & 0 & q^{a^1a^0} & q_{a^1}^{21}+q_{b^1}^{21} & -q_{a^1}^{22}-q_{b^1}^{22}-q^{a^1}-q^{b^1} \\  
	\end{bmatrix}$\ 
	%\end{widetext}
	%\end{multicols}
	%\end{minipage}
	%\end{sideways}
	\caption{Amalgamation Results}
	\label{amalg2}
%\end{figure*}
\end{sidewaysfigure}
\end{proof}
% ------------------------------------------------------------------------

%%% Local Variables: 
%%% mode: latex
%%% TeX-master: "../thesis"
%%% End: 
